# Supplementary material for: A Study on the Impact of Environmental Liability Insurance on Industrial Carbon Emissions
Source: arXiv:2503.15445 source file (2025-03-19)
Supplement: Supplementary file 1 [file supp_alg.tex]

\section{Extended Related Work }
\label{appdx:extended_rw}
\vspace{2mm}

\subsection{Linear Attention}

\paragraph{Feature map $\phi$.} Linear attention mechanisms~\citep{katharopoulos2020transformers} replace $\exp(\vq_t \vk_i^\intercal)$ with a kernel $k(\vx, \vy)$ having an associated feature map $\phi$ (i.e., $k(\vx, \vy) = \langle\phi(\vx), \phi(\vy)\rangle$) where $\phi \in \R^{d_{\text{key}}}\rightarrow \R^{d_{\text{dot}}}$.
$\phi$ often consists of two parts: $\phi = \phi_0 \circ \phi_1$. $\phi_1$ could be a linear map made up by random samples \cite{peng2021random, performer}, learnable MLPs \cite{kasai-etal-2021-finetuning, Hedgehog, polysketch} or simply an identity map \cite{mao-2022-fine}. $\phi_2$ is often an element-wise (activation) function that makes the resulting $\phi$ a positive feature map, such as $1+\operatorname{elu}$ \cite{katharopoulos2020transformers}, $\operatorname{ReLU}$ \cite{kasai-etal-2021-finetuning}, $\exp(\cdot)$ \cite{Hedgehog, performer}. Some work \cite{qin2023scaling, sun2023retentive, mao-2022-fine} suggests that a positive feature map might not be necessary.

Our work follows \citet{sun2023retentive} and \citet{mao-2022-fine} by using an identity map $\phi=\mathbf{I}$.  Recent work suggests that non-identity feature maps such as scaled element-wise exponential map  \cite{log-normal, Hedgehog}
and higher-order polynomial map \cite{Arora2024SimpleLA,polysketch} work well empirically. We leave the exploration of integrating other types of feature map into GLA to future work.

\paragraph{Attention spikiness.} Linear attention suffers from the ``attention dilution'' issue \citep{qin2022devil}, where the attention distribution is too uniform (i.e., high entropy) to concentrate on relevant tokens. \citet{qin2022devil} propose adding local attention layers to focus more on adjacent tokens, a method adopted in \citep{VQ-Transformer, log-normal, orthogonal_memory} and proven crucial for performance. 
Recent work finds that a scaled element-wise exponential map---i.e., $\phi(\mathbf{x})= \mathbf{\exp}(t\cdot \mathbf{x})$ with $t \ge 2$---helps to concentrate attention \cite{log-normal, Hedgehog}. \citet{Hedgehog} also find that higher-order polynomial kernels induce low-entropy and spiky attention distribution, partially explaining the empirical success of Based Linear Attention \cite{Arora2024SimpleLA} and PolySketchFormer \cite{polysketch}.

\paragraph{Memory capacity.} 
 Linear attention has bounded memory size \cite{peng-etal-2022-abc} while softmax attention enjoys unbounded memory\cite{Oren2024TransformersAM}. We believe that increasing the memory size efficiently and utilizing memory effectively are the keys to bridging the performance gap between linear attention and softmax attention. To increase memory size, it is shown that  directly increasing $d_{\operatorname{key}}$ is effective \citep{sun2023retentive, mao-2022-fine, zhang-cai-2022-linearizing}; however, the total parameters are hard to control with the increase of $d_{\operatorname{key}}$.
 Parameter-efficient methods often keep $d_{\text{key}}$ intact and increase $d_{\text{dot}}$ instead. Higher order polynomial kernels with order $p\ge2$ map $d_{\text{key}}$ to a much higher  $d_{\text{dot}} = O(d_\text{key}^p)$ \citep{zoology, polysketch}.  \citet{linear-xmr-fastweight} propose the Deterministic Parameter-Free Projection (DPFP), while \citet{recurrent_linear_xfmr} use parameterized outer product to expand  $d_{\text{dot}}$ in a parameter-efficient/free manner. 
 
 For better memory utilization, \citet{linear-xmr-fastweight} use the delta rule to edit the memory dynamically. However, this is shown to underperform the gating mechanism \cite{mao-2022-fine}, which is a classic method to erase irrelevant historical information in gated RNNs. Recently, \citet{orthogonal_memory} enforce orthogonality of memory vectors to potentially increase utiliziation.

 \paragraph{Linear attention with decay or gates.} \citet{peng2021random} use position-wise scalar gates for incorporating recency bias into linear attention, and has been revisited in recent work \cite{mamba2, beck2024xlstm, Sun2024YouOC},
 while \citet{mao-2022-fine, recurrent_linear_xfmr} use matrix-valued gates (obtained by the outer product) for more fine-grained memory control.

Scalar decays can be easily incorporated into chunkwise linear attention for training efficiency \citep{sun2023retentive, lightning2}. With matrix-valued gates, the training efficiency becomes much more challenging. 
 Both \citet{mao-2022-fine} and \citet{gatedloop}'s training algorithms involve materializing hidden states of all steps in HBM, which  suffers from high I/O costs. Moreover, both approaches cannot take advantage  of tensor cores. Our hardware-efficient training algorithm reduces or eliminates materialization and enables usage of tensor cores.

\paragraph{I/O-aware chunkwise linear attention.} 

The chunkwise form of  linear attention is well-known in the literature.  \citet{GAU} first propose the chunkwise linear attention form, arguing that the training algorithm of \citet{katharopoulos2020transformers} is slow in practice. 
\citet{sun2023retentive} and \citet{lightning2} generalize this form to linear attention with exponential decay (or ALiBi).  \citet{polysketch,VQ-Transformer} also derive similar chunkwise forms.

 However, most chunkwise linear attention is not I/O-aware. To the best of our knowledge, only \textsc{LightningAttention2} \cite{lightning2} (concurrent to our work) is I/O aware, and it is very similar to the non-materialization version of our \textsc{FlashLinearAttention}.  We additionally propose a materialization version, which leverages sequence-level parallelism and thus allows for higher training throughput at the cost of a slightly increasing memory footprint.

\paragraph{Other subquadratic models.} Besides the Linear attention Transformer \cite{katharopoulos2020transformers, linear-xmr-fastweight} discussed in this work, previous studies have explored sparsifying attention with either a predefined fixed pattern \cite{child2019generating, beltagy2020longformer, zaheer2020big} or a context-aware learnable pattern \cite{roy2020efficient, kitaev2020reformer, ren2023sparse} for sequence modeling with subquadratic complexity in the sequence length dimension. Leveraging convolutions for efficient sequence modeling has also been studied in works such as Dynamic Convolution \cite{wu2019pay}, Long Convolution \cite{fu2023simple, qin2023toeplitz, hyena, massaroli2023laughing, li2023what, romero2021ckconv}, and State Space Models \cite{gu2021efficiently, gupta2022diagonal, gu2021combining, hasani2022liquid, s5, ma2023mega}.

\subsection{Sequence parallelism}

The chunk-wise parallel form of linear Transformers resembles the two-stage parallel prefix sum (or parallel scan) algorithm \citep{Blelloch1990PrefixSA}, which also combine chunk-wise parallel computations with inter-chunk communication \citep{Chaurasia2015CompilingHP}.  It also resembles sequence parallelism used for accelerating attention-based Transformers  \citep{li-etal-2023-sequence}, which has recently received  much attention  for long-sequence modeling \citep{Liu2023RingAW, Li2023LightSeqSL, Brandon2023StripedAF}. Sequence-level parallelism also constitutes the main improvement of FlashAttention-2 \citep{flashattention2} over FlashAttention-1 \citep{flashattention1}. The main differences between these works are that (i) the chunk-level parallel form of linear Transformer needs only a single pass due to the linear complexity, while the sequence parallelism in Transformers needs $L/C$ passes (i.e., left-to-right scan of key/value blocks for each query block) due to the inherent quadratic complexity, and (ii) the order of matrix multiplications is different. We also note that chunkwise linear attention could greatly reduce the communication cost between devices in the distributed training setting compared to softmax attention, which could open the door for extremely long sequence training.

\begin{algorithm}[hb]
\scriptsize
\caption{\textsc{FlashLinearAttention}: Backward Pass}
\label{algo:la-chunk-bwd}
\begin{algorithmic}
    \Require $\rmQ, \rmK, \rmV, \rmO, \rmdO \in \R^{L \times d}$, chunk size $C \in [L]$,  \texttt{materialize} $\in$ \{\texttt{True,False}\}, $\rmS \in \R^{\frac{L}{C} \times d \times d}$ \Comment{$\rmS$ is available when \texttt{materialize} is True}
 \State{Initialize $\rmdS = \bm{0} \in \mathbb R^{d\times d} $ on SRAM}
         \State On chip, construct causal mask $\rmM\in \R^{C\times C}$ %
\If{\texttt{materialize}} \Comment{the materialization version}
\color{black}
    \For{$n \gets N, 1$}   \Comment{in reverse order}
        \State Store $\rmdS$ in HBM as $\rmdS_{[n]}$
    \color{black}
        \State{Load $\rmQ_{[n]}, \rmdO_{[n]}  \in \R^{C \times d}$ from HBM to SRAM.}
        \State On chip, compute $\rmdS = \rmdS + \rmQ_{[n]}^\intercal \rmdO_{[n]}$
        \color{orange}
            \color{black}
      \EndFor
      \ParFor{$n \gets 1, N$}  
        \State{Load $\rmQ_{[n]}, \rmK_{[n]},\rmV_{[n]}, \rmdO_{[n]} \in \R^{C \times d}$ from HBM to  SRAM.}
        \State{Load $ \rmS_{[n]}$, $\rmdS_{[n]} \in \R^{d \times d}$ from HBM to SRAM.}

   \State On chip:  $\mathbf{dQ} = \mathbf{dO}_{[n]} \rmS_{[n]}^{\top}  + (\mathbf{dO}_{[n]} \rmV_{[n]}^{\top} \odot \mathbf{M}) \mathbf{K}_{[n]}$.
   \State On chip:   $\mathbf{dK} =  \mathbf{V}_{[n]} \mathbf{dS}_{[n]}^{\top} +  (\mathbf{V}_{[n]}\mathbf{dO}_{[n]}^{\top} \odot \mathbf{M}^{\top}) \mathbf{Q}_{[n]}$
   \State On chip: $\mathbf{dV} =  \mathbf{K}_{[n]} \mathbf{dS}_{[n]} + (\rmQ_{[n]}\rmK_{[n]}^{\top} \odot \mathbf{M})^{\top} \mathbf{dO}_{[n]}$
    \State Write $ \mathbf {dQ}, \mathbf{dK}, \mathbf{dV}$ to HBM as $\mathbf{dQ}_{[n]}, \mathbf{dK}_{[n]}, \mathbf{dV}_{[n]}$
      \EndParFor
      \color{black}
\Else  \Comment{the non-materialization version}
\State Initial $\rmS = \bm{0} \in \mathbb R^{d\times d} $ on SRAM
\For{$n \gets 1, N$}    \Comment{hidden state recomputation}
\State Load $\rmK_{[n]}, \rmV_{[n]}, \rmdO_{[n]}   \in \R^{C \times d}$ from HBM to SRAM.
\State On chip: $\rmdQ = \mathbf{dO}_{[n]} \rmS^{\top}  + (\mathbf{dO}_{[n]} \rmV_{[n]}^{\top} \odot \mathbf{M}) \mathbf{K}_{[n]}$ 
\State On chip: $\rmS = \rmS + \rmK_{[n]}^{\top}\rmV_{[n]}$
\EndFor
\color{black}
    \For{$n \gets N, 1$}   \Comment{in reverse order}
    \color{black}
        \State{Load $\rmQ_{[n]},\rmK_{[n]}, \rmV_{[n]}, \rmdO_{[n]}  \in \R^{C \times d}$ from HBM to SRAM.}
        \State On chip, compute $\rmdS = \rmdS + \rmQ_{[n]}^\intercal \rmdO_{[n]}$
       \State On chip:  $\mathbf{dQ} = \mathbf{dO}_{[n]} \rmS_{[n]}^{\top}  + (\mathbf{dO}_{[n]} \rmV_{[n]}^{\top} \odot \mathbf{M}) \mathbf{K}_{[n]}$.
       \State On chip:   $\mathbf{dK} = \mathbf{V}_{[n]}\mathbf{dS}_{[n]}^{\top}  +  (\mathbf{V}_{[n]}\mathbf{dO}_{[n]}^{\top} \odot \mathbf{M}^{\top}) \mathbf{Q}_{[n]}$
       \State On chip: $\mathbf{dV} =  \mathbf{K}_{[n]} \mathbf{dS}_{[n]} + (\rmQ_{[n]}\rmK_{[n]}^{\top} \odot \mathbf{M})^{\top} \mathbf{dO}_{[n]}$
           \State Write $ \mathbf {dQ}, \mathbf{dK}, \mathbf{dV}$ to HBM as $\mathbf{dQ}_{[n]}, \mathbf{dK}_{[n]}, \mathbf{dV}_{[n]}$
            \color{black}
      \EndFor
\EndIf 
  \State \Return $\rmdQ = \{ \rmdQ_{[1]} \dots \rmdQ_{[N]} \}$, $\rmdK=\{ \rmdK_{[1]} \dots \rmdK_{[N]} \}$, $\rmdV=\{ \rmdV_{[1]} \dots \rmdV_{[N]} \}$.
\end{algorithmic}
\end{algorithm}

\subsection{Hardware-ware algorithm} Many algorithms are fast in theory, but slow in practice, due to misalignment with hardware properties \cite{Hooker2020TheHL,Saphra2023FirstTT}. 
For example, matmuls with butterfly matrices have theoretically lower complexity by using FFT, but in practice it is slow due to extensive memory  transportation operations, motivating matrices  \cite{Dao2022MonarchES,Fu2023MonarchMA} which can better align butterfly operators to GPUs. In practice it is important to reduce HBM I/O cost using techniques such as tiling and recomputation  and leverage tensor cores as much as possible. Our \textsc{FlashLinearAttention} is similar in spirit to \textsc{FlashAttention} \cite{flashattention1,flashattention2} and \textsc{FlashConvFFT} \cite{flashconvfft}, which implement I/O-aware versions of neural network layers to enable practical wallclock speedups. Concurrent work by \citet{lightning2} also proposes an I/O-aware version of linear attention, which is  similar to the non-materialization version of  \textsc{FlashLinearAttention}. We additionally propose a materialization version, which leverages sequence-level parallelism and thus allows for higher training throughput at the cost of a slightly increasing memory footprint.
\label{sec:gla_algo}

\section{Details for Chunkwise (Gated) Linear Attention}
\paragraph{Backward pass of \textsc{FlashLinearAttention}.}  
The pseduocode for backward pass of linear attention is listed in Algorithm~\ref{algo:la-chunk-bwd}.

\paragraph{Pseudo codes of GLA.}
We first present the direct adaptions of \textsc{FlashLinearAttention} to training GLA without secondary-level chunking. 
Specifically, 
Alg.~\ref{algo:gla-chunk-scan-1-fwd} and \ref{algo:gla-chunk-scan-1-bwd} shows the forward/backward pass for the materialization version; Alg.~\ref{algo:gla-chunk-scan-2-fwd} and \ref{algo:gla-chunk-scan-2-bwd} for the non-materialization version.
We show the psuedo code of our secondary-level chunking in Pytorch style in Listing~\ref{a}.

\begin{algorithm}[b!]
\footnotesize
\caption{Forward pass for gated linear attention (w. materialization)}
\label{algo:gla-chunk-scan-1-fwd}
\begin{algorithmic}
    \Require $\rmQ, \rmK, \in \R^{L \times d_k}, \rmV  \in \R^{L \times d_v}$, $\rmG =[\balpha_1 \dots \balpha_L] \in \R^{L \times d_k}$, chunk size $C$
    \State Divide $\rmQ, \rmK, \rmG$ into $N = \frac{L}{C}$ blocks $\{ \rmQ_{[1]} \dots \rmQ_{[N]} \} $, $\{ \rmK_{[1]} \dots \rmK_{[N]} \}$, $\{ \rmG_{[1]} \dots \rmG_{[N]} \} $ of size $C \times d_k$ each.
    \State Divide $\rmV$ into $N$ blocks $\{ \rmV_{[1]} \dots \rmV_{[N]} \}$ of size $C \times d_v$ each.
     \State{Initialize $\rmS = \bm{0} \in \mathbb R^{d_k\times d_v} $ on SRAM}
    \For{$n \gets 1, N$}
      \State{Write $\mathbf S$ to HBM as $\rmS_{[n]}$.} 
        \State Load $\rmK_{[n]}, \rmG_{[n]} \in \R^{C \times d_k}$ from HBM to SRAM. 
        \State Load $\rmV_{[n]} \in \R^{C \times d_v}$ from HBM to SRAM.
        \State On chip, compute $\bgamma_{[n]} \in \R^{d_k}, \bGamma_{[n]} \in \R^{C \times d_k}$ and $\tilde \rmK_{[n]} = \rmK_{[n]} \odot \bGamma_{[n]}$. %
        \State{On chip, compute $\rmS = \left(\bgamma_{[n]}^\intercal\mathbf{1}\right) \odot \mathbf{S} + \tilde \rmK_{[n]}^{\top}  \rmV_{[n]}$.}  
    \EndFor
   \ParFor{$n \gets 1, N$}
        \State Load $\rmQ_{[n]}, \rmK_{[n]}, \rmG_{[n]} \in \R^{C \times d_k}$ from HBM to SRAM.
        \State Load $\rmV_{[n]}  \in \R^{C \times d_v}$ from HBM to SRAM.
        \State Load $\rmS_{[n]} \in \R^{d_k \times d_v}$ from HBM to SRAM.
        \State On chip, construct causal mask $\rmM\in \R^{C \times C}$ %
        \State On chip, compute $\bLambda_{[n]}, \bGamma_{[n]} \in \R^{C \times d_k}$
        \State On chip, compute $\tilde \rmQ_{[n]} = \rmQ_{[n]} \odot \bLambda_{[n]}$, $\tilde \rmK_{[n]} = \rmK_{[n]} \odot \bGamma_{[n]}$, $\bar \rmK_{[n]} = \rmK_{[n]} / \bLambda_{[n]}$
        \State On chip, compute $\rmO_{[n]}^{\text{inter}} = \tilde \rmQ_{[n]} \rmS_{[n]} \in \R^{C \times d_v}$
        \State On chip, compute $\rmP = (\tilde \rmQ_{[n]} \bar \rmK^\intercal_{[n]})\odot \rmM  \in \R^{C \times C} $
        \State On chip, compute $\rmO^{\text{intra}} = \rmP \rmV_{[n]} $ 
        \State On chip, compute $ \rmO_{[n]} = \rmO^{\text{inter}} + \rmO^{\text{intra}} $
        \State Store $\rmO_{[n]}$ to HBM.
   \EndParFor
  \State \Return $\rmO = \{ \rmO_{[1]} \dots \rmO_{[N]} \}$, $\rmS=\{ \rmS_{[1]} \dots \rmS_{[N]} \}$.
\end{algorithmic}
\end{algorithm}
\begin{algorithm}[tbh!]
\footnotesize
\caption{Backward pass for gated linear attention (w. materialization)}
\label{algo:gla-chunk-scan-1-bwd}
\begin{algorithmic}
    \Require $\rmQ, \rmK, \rmG \in \R^{L \times d_k}$, $\rmV, \rmO, \rmdO \in \R^{L \times d_v}$, chunk size $C$
     \State{Initialize $\rmdS = \bm{0} \in \mathbb R^{d_k\times d_v} $ on SRAM}
    \For{$n \gets N, 1$} %
        \State Store $\rmdS$ in HBM as $\rmdS_{[n]}$
        \State{Load $\rmG_{[n]}  \in \R^{C \times d_k}$ from HBM to SRAM.}
        \State{Load $\rmQ_{[n]}  \in \R^{C \times d_k}$ from HBM to SRAM.}
        \State{Load $\rmdO_{[n]}  \in \R^{C \times d_v}$ from HBM to SRAM.}
        \State On chip, compute $\bgamma_{[n]}$, $\bGamma_{[n]}$ and $\tilde \rmQ{[n]} =  \rmQ_{[n]} \odot \bGamma{[n]}$
        \State On chip, compute $\rmdS = \left(\bgamma_{[n]}^\intercal\mathbf{1}\right) \odot \rmdS + \tilde \rmQ_{[n]}^\intercal \rmdO_{[n]}$
      \EndFor
      \ParFor{$n \gets 1, N$}
        \State{Load $\rmQ_{[n]}, \rmK_{[n]}, \rmG_{[n]} \in \R^{C \times d_k}$ from HBM to  SRAM.}
        \State Load $\rmS_{[n]} \in \R^{d_k \times d_v}$ from HBM to  SRAM.
        \State Load $\rmV_{[n]}, \rmO_{[n]}, \rmdO_{[n]} \in \R^{C \times d_v}$ from HBM to  SRAM.
        \State Load $\rmdS_{[n]} \in \R^{d_k \times d_v}$ from HBM to SRAM.
        \State On chip, construct causal mask $\rmM\in \R^{B\times B}$ %
        \State On chip, compute $\bLambda_{[n]}, \bGamma_{[n]} \in \R^{C \times d_k}$
        \State On chip, compute $\tilde \rmQ_{[n]} = \rmQ_{[n]} \odot \bLambda_{[n]}$, $\tilde \rmK_{[n]} = \rmK_{[n]} \odot \bGamma_{[n]}$, $\bar \rmK_{[n]} = \rmK_{[n]} / \bLambda_{[n]}$.
        \State On chip, compute $\rmP = (\tilde \rmQ_{[n]} \tilde \rmK^\intercal_{[n]})\odot \rmM  \in \R^{C \times C} $
        \State On chip, compute $\rmdP =( \rmdO_{[n]} \rmV_{[n]}^\intercal) \odot \rmM $
        \State On chip, compute $ \rmdbK_{[n]} = \tilde \rmQ_{[n]} \rmdP^\intercal$
        \State On chip, compute $ \rmdtK_{[n]} = \rmV_{[n]} \rmdS_{[n]}  ^\intercal$
        \State On chip, compute $\rmdK_{[n]} =  \rmdtK_{[n]} \odot \bGamma_{[n]}  + \rmdbK_{[n]} / \bLambda_{[n]} $
        \State{On chip, compute $\rmdtQ_{[n]} = \rmdP \, \bar \rmK_{[n]} + \rmdO_{[n]} \rmS_{[n]}^\intercal $}
        \State On chip, compute $\rmdQ_{[n]} =  \rmdtQ_{[n]} \odot \bLambda_{[n]} $
        \State On chip, compute $\rmdV_{[n]} = \rmP^\intercal \, \rmdO_{[n]} + \tilde \rmK_{[n]} \rmdS_{[n]} $
        \State Store $\rmdK_{[n]}, \rmdV_{[n]}$ in HBM.
      \EndParFor
  \State Let $\rmdQ = \{ \rmdQ_{[1]} \dots \rmdQ_{[N]} \}$, $\rmdK=\{ \rmdK_{[1]} \dots \rmdK_{[N]} \}$, $\rmdV=\{ \rmdV_{[1]} \dots \rmdV_{[N]} \}$.
  \State Compute $\rmdA = \rmQ \odot \rmdQ - \rmK \odot \rmdK $, $\rmdG = \revcum(\rmdA) $
  \State \Return $\rmdQ, \rmdK, \rmdV, \rmdG$
\end{algorithmic}
\end{algorithm}

\begin{algorithm}[b!]
\small
\caption{Forward pass for gated linear attention (w/o. materialization)}
\label{algo:gla-chunk-scan-2-fwd}
\begin{algorithmic}
    \Require $\rmQ, \rmK, \in \R^{L \times d_k}, \rmV  \in \R^{L \times d_v}$, $\rmG =[\balpha_1 \dots \balpha_L] \in \R^{L \times d_k}$, chunk size $C$
    \State Divide $\rmQ, \rmK, \rmG$ into $N = \frac{L}{B}$ blocks $\{ \rmQ_{[1]} \dots \rmQ_{[N]} \} $, $\{ \rmK_{[1]} \dots \rmK_{[N]} \}$, $\{ \rmG_{[1]} \dots \rmG_{[N]} \} $ of size $C \times d_k$ each.
    \State Divide $\rmV$ into $N$ blocks $\{ \rmV_{[1]} \dots \rmV_{[N]} \}$ of size $C \times d_v$ each.
     \State{Initialize $\rmS = \bm{0} \in \mathbb R^{d_k\times d_v} $ on SRAM}
    \For{$n \gets 1, N$}
      \State{Write $\mathbf S$ to HBM as $\rmS_{[n]}$.} 
        \State Load $\rmQ_{[n]}, \rmK_{[n]}, \rmG_{[n]} \in \R^{C \times d_k}$ from HBM to SRAM.
        \State Load $\rmV_{[n]}  \in \R^{C \times d_v}$ from HBM to SRAM.
        \State On chip, compute $\bgamma_{[n]} \in \R^{d_k}, \bGamma_{[n]} \in \R^{C \times d_k}$ and $\tilde \rmK_{[n]} = \rmK_{[n]} \odot \bGamma_{[n]}$. %
        \State On chip, construct causal mask $\rmM\in \R^{C\times C}$ %
        \State On chip, compute $\bLambda_{[n]}, \bGamma_{[n]} \in \R^{C \times d_k}$
        \State On chip, compute $\tilde \rmQ_{[n]} = \rmQ_{[n]} \odot \bLambda_{[n]}$, $\tilde \rmK_{[n]} = \rmK_{[n]} \odot \bGamma_{[n]}$, $\bar \rmK_{[n]} = \rmK_{[n]} / \bLambda_{[n]}$.
        \State On chip, compute $\rmO_{[n]}^{\text{inter}} = \tilde \rmQ_{[n]} \rmS_{[n]} \in \R^{C \times d_v}$
        \State On chip, compute $\rmP = (\tilde \rmQ_{[n]} \bar \rmK^\intercal_{[n]})\odot \rmM  \in \R^{C \times C} $
        \State On chip, compute $\rmO^{\text{intra}} = \rmP \rmV_{[n]} $
        \State On chip, compute $ \rmO_{[n]} = \rmO^{\text{inter}} + \rmO^{\text{intra}} $
        \State Store $\rmO_{[n]}$ to HBM.
        \State{On chip, compute $\rmS = \left(\bgamma_{[n]}^\intercal \mathbf{1}\right) \odot \mathbf{S} + \tilde \rmK_{[n]}^{\top}  \rmV_{[n]}$.}  
   \EndFor
  \State \Return $\rmO = \{ \rmO_{[1]} \dots \rmO_{[N]} \}$.
\end{algorithmic}
\end{algorithm}

\begin{algorithm}[tbh!]
\small
\caption{Backward pass for gated linear attention (w/o. materialization)}
\label{algo:gla-chunk-scan-2-bwd}
\begin{algorithmic}
    \Require $\rmQ, \rmK, \rmG \in \R^{L \times d_k}$, $\rmV, \rmO, \rmdO \in \R^{L \times d_v}$, chunk size $C$
    \State{Initialize $\rmS = \bm{0} \in \R^{d_k\times d_v} $ on SRAM}
    \For{$n \gets 1, N$} %
        \State{Load $\rmG_{[n]}  \in \R^{C \times d_k}$ from HBM to SRAM.}
        \State{Load $\rmQ_{[n]}  \in \R^{C \times d_k}$ from HBM to SRAM.}
        \State{Load $\rmdO_{[n]}  \in \R^{C \times d_v}$ from HBM to SRAM.}
        \State On chip, compute $\bgamma_{[n]} \in \R^{d_k}, \bGamma_{[n]} \in \R^{C \times d_k}$ and $\tilde \rmK_{[n]} = \rmK_{[n]} \odot \bGamma_{[n]}$.
        \State On chip, compute $\rmdP = \rmdO_{[n]} \rmV_{[n]}^\intercal $
        \State{On chip, compute $\rmdtQ_{[n]} = \rmdP \, \tilde \rmK_{[n]} + \rmdO_{[n]} \rmS^\intercal $}
        \State On chip, compute $\rmdQ= \rmdtQ_{[n]} \odot \bGamma{[n]} $
        \State Store $\rmdQ_{[n]}$ to HBM.
        \State{On chip, compute $\rmS = \left(\bgamma_{[n]}^\intercal\mathbf{1}\right) \odot \mathbf{S} + \tilde \rmK_{[n]}^{\top}  \rmV_{[n]}$.}  
      \EndFor
    \State{Initialize $\rmdS = \bm{0} \in \mathbb R^{d_k\times d_v} $ on SRAM}
      \For{$n \gets N, 1$}
        \State{Load $\rmQ_{[n]}, \rmK_{[n]}, \rmG_{[n]} \in \R^{C \times d_k}$ from HBM to  SRAM.}
        \State Load $\rmV_{[n]}, \rmO_{[n]}, \rmdO_{[n]} \in \R^{C \times d_v}$ from HBM to  SRAM.
        \State On chip, construct causal mask $\rmM\in \R^{C\times C}$ %
        \State On chip, compute $\bLambda_{[n]}, \bGamma_{[n]} \in \R^{C \times d_k}$
        \State On chip, compute $\tilde \rmQ_{[n]} = \rmQ_{[n]} \odot \bLambda_{[n]}$, $\tilde \rmK_{[n]} = \rmK_{[n]} \odot \bGamma_{[n]}$.
        \State On chip, compute $\rmP = (\tilde \rmQ_{[n]} \tilde \rmK^\intercal_{[n]})\odot \rmM  \in \R^{C \times C} $
        \State On chip, compute $\rmdP = (\rmdO_{[n]} \rmV_{[n]}^\intercal) \odot \rmM $
                \State On chip, compute $ \rmdbK_{[n]} = \tilde \rmQ_{[n]} \rmdP^\intercal$
        \State On chip, compute $ \rmdtK_{[n]} = \rmV_{[n]} \rmdS_{[n]}  ^\intercal$
        \State On chip, compute $\rmdK_{[n]} =  \rmdtK_{[n]} \odot \bGamma_{[n]}  + \rmdbK_{[n]} / \bLambda_{[n]} $
        \State On chip, compute $\rmdV_{[n]} = \rmP^\intercal \, \rmdO_{[n]} + \tilde \rmK_{[n]} \rmdS $
        \State Store $\rmdQ_{[n]}, \rmdK_{[n]}, \rmdV_{[n]}$ in HBM.
        \State On chip, compute $\rmdS = \left(\bgamma_{[n]}^\intercal \mathbf{1} \right) \odot \rmdS + \tilde \rmQ_{[n]}^\intercal \rmdO_{[n]}$
      \EndFor
  \State Let $\rmdQ = \{ \rmdQ_{[1]} \dots \rmdQ_{[N]} \}$, $\rmdK=\{ \rmdK_{[1]} \dots \rmdK_{[N]} \}$, $\rmdV=\{ \rmdV_{[1]} \dots \rmdV_{[N]} \}$.
  \State Compute $\rmdA = \rmQ \odot \rmdQ - \rmK \odot \rmdK $, $\rmdG = \revcum(\rmdA) $
  \State \Return $\rmdQ, \rmdK, \rmdV, \rmdG$
\end{algorithmic}
\end{algorithm}

\paragraph{Derivations of $\dblogalpha_t$.}

We show the derivations for the following gradient form.
\begin{align*}
    \vdlogb_t &= \vk_t \odot \vdk_t - \vq_t \odot \vdq_t, \\
   \dblogalpha_t  &= \sum_{t \leq i \leq L} \vdlogb_i.
\end{align*}

By unrolling the recurrence, we have
\begin{align*}
\vo_t =  \vq_t \rmS_t  &= \sum_{i=1}^{t}(\vq_t \odot \vb_t) \left(\frac{\vk_i}{\vb_i}\right)^{\top} \vv_i \\
&=  \sum_{i=1}^{t}(\vq_t \odot \exp(\log \vb_t)) \left(\vk_i \odot {\exp(- \log \vb_i)}\right)^{\top} \vv_i
\end{align*}
where at the second step, we apply a trivial identity: $\exp(\log x) = x$.
We first derive the gradients wrt. query/key vectors,
\begin{align*}
& \vdq_t = \sum_{ i = 1}^{t} \langle \vdo_t, \vv_i\rangle  \vb_t \odot \vk_i / \vb_i,  \\
& \vdk_i = \sum_{t = i}^{L} \langle \vdo_t, \vv_i\rangle  \vq_t \odot  \vb_t  / \vb_i.
\end{align*}
Then for the gradients wrt. the logits of the accumulative gates,
\begin{align*}
& \vdlogb_t  = \vq_t \odot \underbrace{\sum_{i=1}^{t} \langle \vdo_t, \vv_i\rangle  \odot  \vb_t  \odot  \vk_i / \vb_i}_{  \vdq_t} - \vk_t \odot \underbrace{\sum_{i = t}^{L} \langle \vdo_i, \vv_t\rangle  \vq_i \odot  \vb_i  / \vb_t}_{\vdk_t}.
\end{align*}
where we change the index notation for the $\vdk$ term.
It now becomes clear that 
\begin{align*}
& \vdlogb_t =  \vq_t \odot \vdq_t  - \vk_t \odot \vdk_t.
\end{align*}
Since $\vlogb_t = \sum_{i=1}^t \vlogalpha_i$, we get $\dblogalpha_t  = \sum_{t = i}^L \vdlogb_i$.
