# Supplementary material for: A Study on the Impact of Environmental Liability Insurance on Industrial Carbon Emissions
Source: arXiv:2503.15445 source file (2025-03-19)
Supplement: Supplementary file 2 [file supp_method.tex]

\section{General Gated Linear Attention}
\label{sec:ggla}

In the main paper, we use a simplified parameterization where $\bbeta$ is fixed to $\mathbf{1}$ in the following gated linear attention.
\begin{align*}
\rmS_t = (\balpha_t^{\top} \bbeta_t) \odot \rmS_{t-1} + \vk_t^{\top} \vv_t,
\end{align*}
Though empirically we found that making $\bbeta$ learnable does not lead to performance gain, we show here that the general form still enjoys parallel form and chunk-wise form, which could be potentially useful for future development of linear attention models.

\subsection{Parallel form}

By unrolling the recurrence we have,
\begin{align}
\vo_t = \vq_t \rmS_t 
= \vq_t \sum_{i=1}^{t} \big((\prod_{i+1}^{t} \rmG_{i}) \odot (\vk_i^{\intercal}\vv_i)\big) 
\end{align}

By taking advantage of the mixed product property of Kronercker/outer product, we have
\begin{align}
(\prod_{j=i+1}^{t} \rmG_j) \odot (\vk_i^{\intercal} \vv_i) &= \big((\frac{\vb_t}{\vb_i})^{\intercal}(\frac{\vd_t}{\vd_i})\big) \odot (\vk_i^{\intercal} \vv_i) \\
&=\left( \frac{\vb_t}{\vb_i}\odot \vk_i \right)^{\intercal} \left( \frac{\vd_t}{\vd_i} \odot \vv_i \right) 
\end{align}
where $\vb_t = \prod_{j=1}^t \balpha_j, \vd_t = \prod_{j=1}^t \bbeta_j$.
By plugging it into the expanded recurrence, we have the following form. 
\begin{align}
\vo_t = \vq_t \rmS_t 
&= 
\vq_t \sum_{i=1}^{t} \big((\prod_{i+1}^{t} \rmG_{i}) \odot (\vk_i^{\intercal}\vv_i)\big) \\
    &= \vq_t \sum_{i=1}^{t} \left( \frac{\vb_t}{\vb_i}\odot \vk_i \right)^{\intercal} \left( \frac{\vd_t}{\rmB_i} \odot \vv_i \right) \\ 
    &= \sum_{i=1}^{t} \left(\vq_t \left( \frac{\vb_t}{\vb_i}\odot \vk_i \right)^{\intercal}\right) \left( \frac{\vd_t}{\vd_i} \odot \vv_i \right) \label{eq:gla_parallel_1} \\
    &= \sum_{i=1}^{t} \underbrace{\left\langle \vq_t, \frac{\vb_t}{\vb_i} \odot \vk_t \right\rangle}_{\R^{1\times 1}} \underbrace{\left( \frac{\vd_t}{\vd_i} \odot \vv_t \right)}_{\mathbb{R}^{1\times d_v}}  \\    
    &= \sum_{i=1}^{t} \left(\left\langle \vq_t \odot \vb_t, \frac{\vk_i}{\vb_i}\right\rangle \frac{\vv_i}{\vd_i} \right) \odot \vd_t \qquad  \label{eq:gla_parallel_2} \\
    &= \sum_{i=1}^{t} \left( \left(\vq_t \odot \vb_t\right)\left(\frac{\vk_i}{\vb_i}\right)^{\intercal} \left(
    \frac{\vv_i}{\vd_i} \right) \right) \odot \vd_t \quad \in \mathbb{R}^{1\times d_v} 
\end{align}
Eq.~\ref{eq:gla_parallel_1} is by linearity and associative property of matrix multiplication, Eq.~\ref{eq:gla_parallel_2} is derived based on $\langle \va, \vb \odot \vc \rangle = \langle \va \odot \vb, \vc \rangle$. The final form has following equivalent parallel form similar to the parallel form of linear/softmax attention.
\begin{align}
    \tilde \rmQ &= \rmQ \odot \rmB \qquad \tilde \rmK = \rmK / \rmB \qquad \tilde \rmV = \rmV / \rmD \\
    \tilde \rmO &= (\tilde \rmQ \tilde \rmK^\intercal \odot \rmM) \tilde \rmV \qquad \rmO = \tilde \rmO \odot \rmD
    \label{eq:gla_QKV}
\end{align}
where $\rmQ, \rmK, \rmB \in \R^{L \times d_k}$,
 $\rmV, \rmD \in \R^{L \times d_v}$,
 $\rmM \in \R^{L \times L}$ denotes the causal mask.

\subsection{Chunkwise parallel form}

Now we show that the chunkwise parallel form for efficient training of general linear attention. Suppose $\rmX$ is now split into $\frac{L}{C}$ chunks, each of length $C$. Let $\rmS_{[i]} \in \R^{d_k \times d_v}$ be the chunk-level hidden state after processing $i$ chunks, i.e., $\rmS_{[i]}:=\rmS_{iC}$. Further let $\rmK_{[i+1]}:=\rmK_{iC+1:(i+1)C} \in \mathbb{R}^{C\times d_k}$, $\rmV_{[i+1]}:=\rmV_{iC+1:(i+1)C} \in \mathbb{R}^{C\times d_v}$. The inter-chunk recurrence is then given by,
\begin{align*}
\rmS_{[i+1]} 
&= \left(\Big(\frac{\rmB_{(i+1)C}}{\rmB_{iC}}\Big)^{\intercal}\Big(\frac{\rmD_{(i+1)C}}{\rmD_{iC}}\Big) \right) \odot \rmS_{[i]} +  \big(\rmB^{\prime}_{[i+1]} \odot \rmK_{[i+1]}\big)^{\intercal} \big(\rmD^{\prime}_{[i+1]} \odot \rmV_{[i+1]}\big),
\label{eq:gla_inter_chunk_recur}
\end{align*}
 where $(\rmB^{\prime}_{[i+1]})_j = \frac{\rmB_{(i+1)C}}{\rmB_{iC+j}} \in \mathbb{R}^{1\times d_k}$ and $(\rmD^{\prime}_{[i+1]})_j = \frac{\rmD_{(i+1)C}}{\rmD_{iC+j}} \in \mathbb{R}^{1\times d_v}$ for $j\in [1, C]$, $i \in [0, L/C-1]$. (Therefore we have $\rmB^{\prime}_{[i+1]} \in \R^{C \times d_k}, \rmD^{\prime}_{[i+1]} \in \R^{C \times d_v}$.) The intra-chunk parallel computation is then given by,
\begin{align}
\tilde \rmO_{[i+1]} &= \underbrace{\left((\rmQ_{[i+1]} \odot \rmB^{\dagger}_{[i+1]}) \rmS_{[i]} \right) \odot \rmD^{\dagger}_{[i+1]}}_{\text{inter-chunk}} + \underbrace{
(\tilde\rmQ_{[i+1]} \tilde\rmK_{[i+1]}^{\intercal} \odot \rmM)\tilde\rmV_{[i+1]}
}_{\text{intra-chunk}}, \\ &\rmO_{[i+1]}  = \tilde \rmO_{[i+1]} / \rmD^{\dagger}_{[i+1]},
\label{eq:gla_inter_intra} 
\end{align}
 where $(\rmB_{[i+1]}^{\dagger})_j = \frac{\rmB_{iC+j}}{\rmB_{iC}} \in \mathbb{R}^{1\times d_k}$ and $(\rmD_{[i+1]}^{\dagger})_j = \frac{\rmD_{iC+j}}{\rmD_{iC}} \in \mathbb{R}^{1\times d_v}$  for $j\in [1, C]$, $i \in [0, L/C-1]$. 
 Subsequently, we have $\tilde\rmQ_{[i+1]}=\rmQ_{[i+1]} \odot \rmB_{[i+1]}^{\dagger}, \tilde\rmK_{[i+1]}=\frac{\rmK_{[i+1]}}{\rmB_{[i+1]}^{\dagger}}, \tilde\rmV_{[i+1]}=\rmV_{[i+1]} \odot \rmD_{[i+1]}^{\dagger} $. For initial values, we set $\rmS_0 = \vzero$, $\rmB_0=\mathbf{1}$, $\rmD_0=\mathbf{1}$. Intuitively, $\rmB^{\prime}_{[i]} $ encodes the cumulative decay from the start of a chunk which will be used to propagate the hidden states from the previous chunk $\rmS_{[i]}$;   $\rmB^{\dagger}_{[i]}$ encodes the decay to the end of a chunk which will be used to accumulate information to be added to the next hidden state $\rmS_{[i+1]}$.

The chunkwise form given here is a generalization of several existing forms for linear attention. If we set $\rmA_{ij}=1$, $\rmB_{ij} = 1$, it reduces to the chunk-wise form presented in the main paper for vanilla linear attention; if we set $\rmA_{ij}=1$, $\rmB_{ij} = \gamma^{i+1}$, it becomes RetNet's chunk-wise form \citep{sun2023retentive}. As such, our formulation can be regarded as a generalized chunk-wise parallel form for linear attention that enables fine-grained data-dependent decay. 
\paragraph{Memory-efficient computation of $\dbalpha$ and $\dbbeta$}

In the general form, we show that the gradient wrt. $\balpha$  and $\bbeta$ admits the following closed form, which allows computing $\dbalpha$ and $\dbbeta$ without instantiating $\rmS$ in HBM.
\begin{align*}
    \vdlogb_t &= \vk_t \odot \vdk_t - \vq_t \odot \vdq_t, \\
   \dblogalpha_t  &= \sum_{t \leq i \leq L} \vdlogb_i \\
   \vdlogd_t &= \vo_t \odot \vdo_t - \vv_t \odot \vdv_t, \\
   \dblogbeta_t  &= \sum_{t \leq i \leq L} \vdlogd_i.
\end{align*}
where  $\vlogb_t = \sum_{i=1}^t \log \balpha_i$, $\vlogd_t = \sum_{i=1}^t \bbeta_i$ (or alternatively $\vb_t = \prod_{i=1}^t \balpha_i$, $\vd_t = \prod_{i=1}^t \bbeta_i$).  We apply the trick to compute $\vdlogb_t$ and $\vdlogd_t$ for the following cumulative-sum form.

\begin{align*}
    \vo_t = \sum_{i=1}^{t} \left( \left(\vq_t \odot \vb_t\right)\left(\frac{\vk_i}{\vb_i}\right)^{\intercal} \left(
    \frac{\vv_i}{\vd_i} \right) \right) \odot \vd_t \quad \in \mathbb{R}^{1\times d_v}.
\end{align*}
The gradient of $\vlogb_t$ comes from two sources: one associated with $\vq_t$, the other associated with $\vk_i$. Similarly, $\vlogd_t$ comes from both $\vo_t$ and $\vv_i$.
\begin{align*}
\vdlogb_t  &= \vq_t \odot \underbrace{\sum_{i=1}^{t} \langle \vdo_t, \frac{\vd_t}{\vd_i} \vv_i \rangle  \odot  \vb_t  \odot  \vk_i / \vb_i}_{  \vdq_t} - \vk_t \odot \underbrace{\sum_{i = t}^{L} \langle \vdo_i, \frac{\vd_i}{\vd_t} \vv_t \rangle  \vq_i \odot  \vb_i  / \vb_t}_{\vdk_t} \\
\vdlogd_t  &= \vdo_t \odot \underbrace{\sum_{i=1}^{t} \left( \left(\vq_t \odot \vb_t\right)\left(\frac{\vk_i}{\vb_i}\right)^{\intercal} \left(
    \frac{\vv_i}{\vd_i} \right) \right) \odot \vd_t}_{\vo_t} - \vv_t \odot \underbrace{\sum_{i=t}^{L} \left( \left(\vq_i \odot \vb_i\right)\left(\frac{\vk_t}{\vb_t}\right)^{\intercal} \left(
    \frac{1}{\vd_t} \right) \right) \odot \vd_i}_{\vdv_t} 
\end{align*}
The trick applied there is that $\frac{\partial f(\va \odot \vb )}{\partial \vlogb} = \va \odot \frac{\partial f(\va \odot \vb )}{\partial \va}$ and  $\frac{\partial f(\va / \vb )}{\partial \vlogb}  = - \frac{\partial f(\va / \vb )}{\partial \va} \odot \va $.
