# Supplementary material for: A Study on the Impact of Environmental Liability Insurance on Industrial Carbon Emissions
Source: arXiv:2503.15445 source file (2025-03-19)
Supplement: Supplementary file 3 [file supp_mqar.tex]

\vspace{-2mm}
\section{Additional Experimental Results}
\label{app:d}

The complete results on all 11 tasks, including the 5-shot results for the 1.3B models, are shown in
